# Supplementary material for: 3D GAN Inversion with Pose Optimization
Source: arXiv:2210.07301 source file (2022-10-17)
Supplement: Supplementary file 3 [file catedit.tex]

\begin{figure}[!p]
\centering
\newcolumntype{M}[1]{>{\centering\arraybackslash}m{#1}}
\setlength{\tabcolsep}{1pt}

\begin{tabular}{M{0.1\linewidth}M{0.1\linewidth}M{0.1\linewidth}
@{\hskip 0.01\linewidth} M{0.1\linewidth}M{0.1\linewidth}M{0.1\linewidth} @{\hskip 0.01\linewidth} M{0.1\linewidth}M{0.1\linewidth}M{0.1\linewidth}}

& \includegraphics[width=\linewidth]{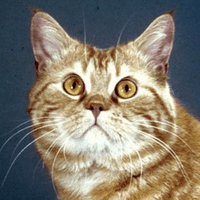}\hfill &
&& \includegraphics[width=\linewidth]{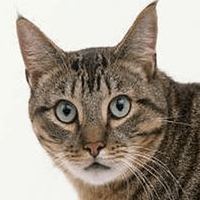}\hfill &
&& \includegraphics[width=\linewidth]{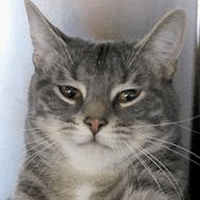}\hfill \\

\includegraphics[width=\linewidth]{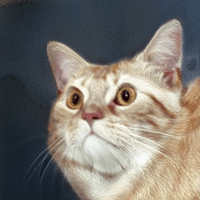}\hfill &
\includegraphics[width=\linewidth]{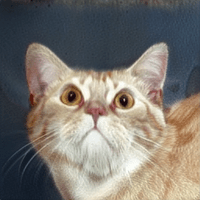}\hfill&
\includegraphics[width=\linewidth]{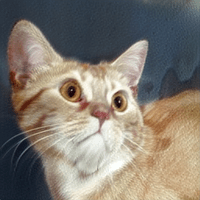}\hfill &

\includegraphics[width=\linewidth]{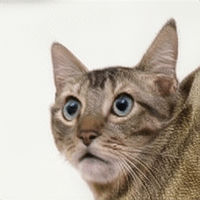}\hfill &
\includegraphics[width=\linewidth]{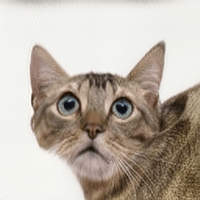}\hfill&
\includegraphics[width=\linewidth]{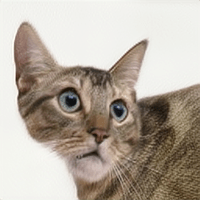}\hfill &

\includegraphics[width=\linewidth]{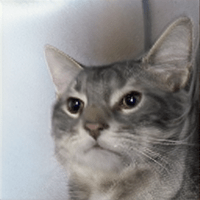}\hfill &
\includegraphics[width=\linewidth]{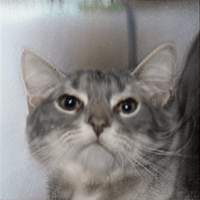}\hfill&
\includegraphics[width=\linewidth]{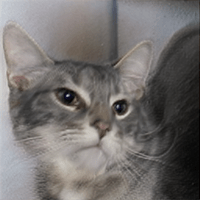}\hfill \\

\includegraphics[width=\linewidth]{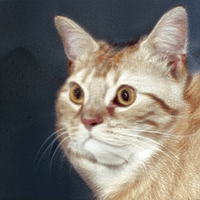}\hfill &
\includegraphics[width=\linewidth]{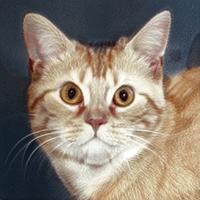}\hfill \llap{\includegraphics[trim=650 130 400 90,clip,width=0.5\linewidth, height=\linewidth]{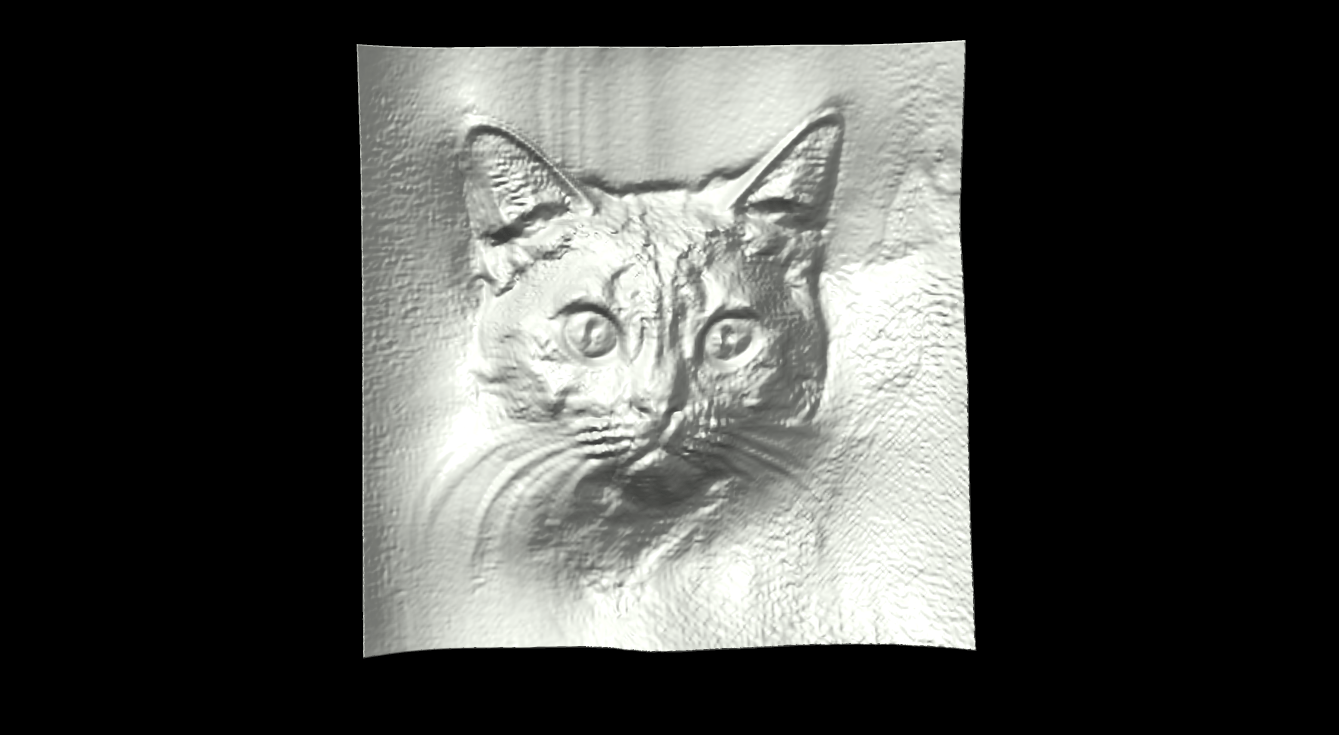}}&
\includegraphics[width=\linewidth]{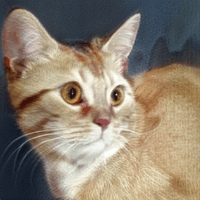}\hfill & 

\includegraphics[width=\linewidth]{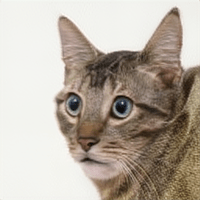}\hfill &
\includegraphics[width=\linewidth]{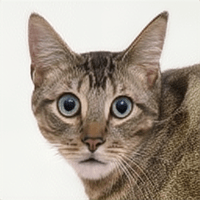}\hfill \llap{\includegraphics[trim=650 130 400 90,clip,width=0.5\linewidth, height=\linewidth]{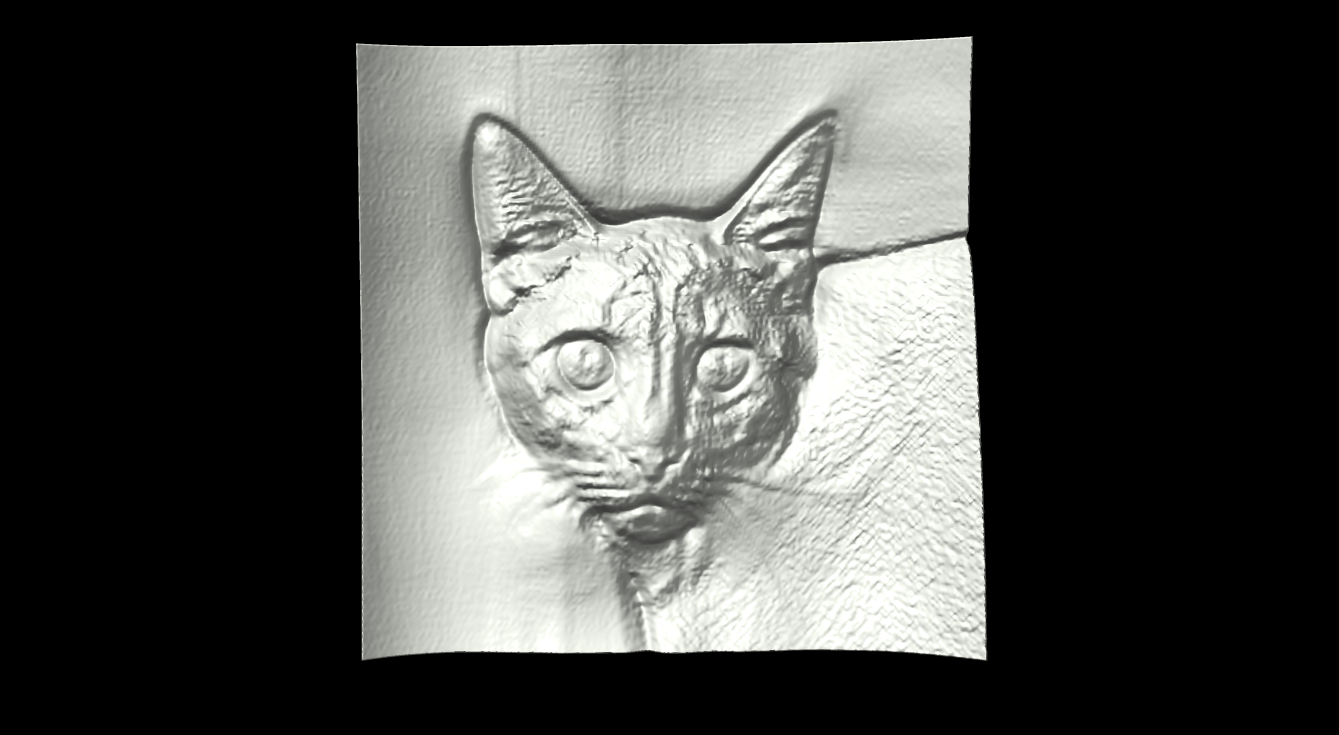}}&
\includegraphics[width=\linewidth]{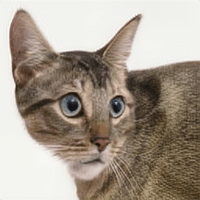}\hfill & 

\includegraphics[width=\linewidth]{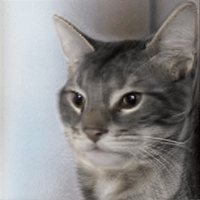}\hfill &
\includegraphics[width=\linewidth]{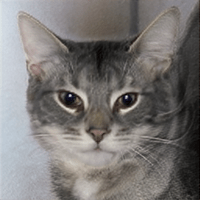}\hfill \llap{\includegraphics[trim=650 130 390 90,clip,width=0.5\linewidth, height=\linewidth]{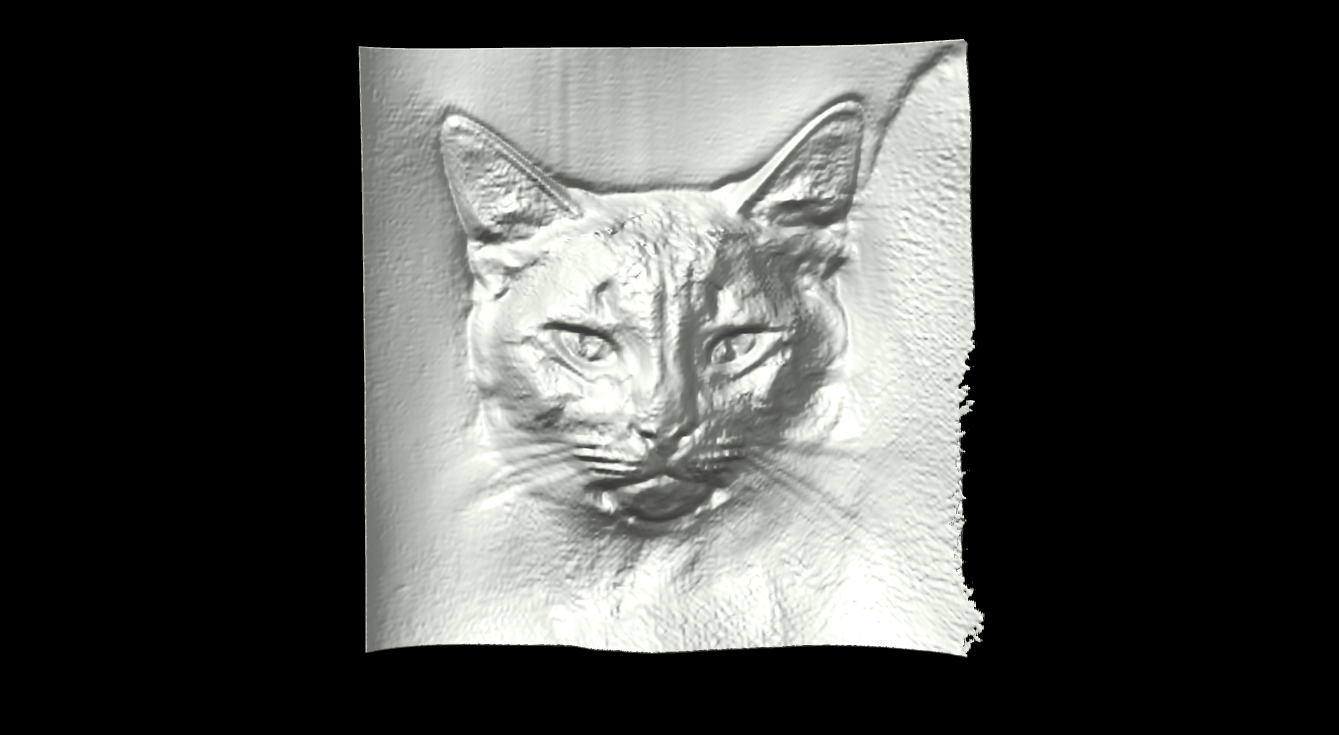}}&
\includegraphics[width=\linewidth]{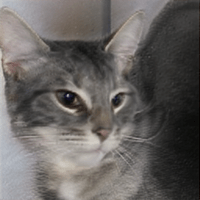}\hfill \\

\includegraphics[width=\linewidth]{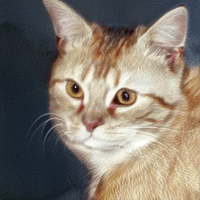}\hfill &
\includegraphics[width=\linewidth]{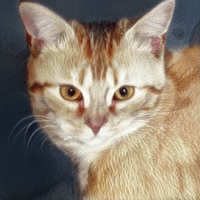}\hfill &
\includegraphics[width=\linewidth]{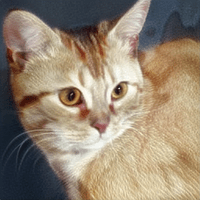}\hfill &

\includegraphics[width=\linewidth]{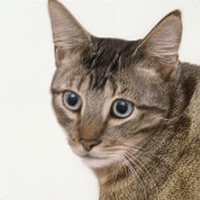}\hfill &
\includegraphics[width=\linewidth]{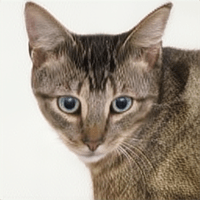}\hfill &
\includegraphics[width=\linewidth]{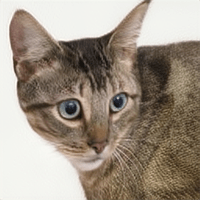}\hfill &

\includegraphics[width=\linewidth]{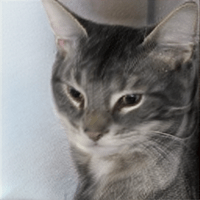}\hfill &
\includegraphics[width=\linewidth]{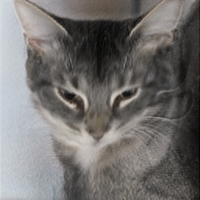}\hfill &
\includegraphics[width=\linewidth]{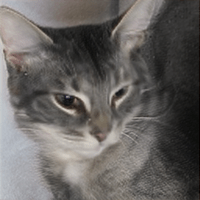}\hfill \\\\\\
\end{tabular}
\caption{\textbf{Latent based editing of 3D shape on AnimalFace10 dataset}}
\label{fig:simultaneous editing}
\end{figure}
